# Supplementary material for: Space-Filling One-Factor-At-A-Time Designs
Source: arXiv:2606.02533 source file (2026-10-06)
Supplement: Supplementary file 1 [file supplementary.tex]

\documentclass[12pt]{article}

% DON'T change margins - should be 1 inch all around.
\addtolength{\oddsidemargin}{-.5in}%
\addtolength{\evensidemargin}{-1in}%
\addtolength{\textwidth}{1in}%
\addtolength{\textheight}{1.7in}%
\addtolength{\topmargin}{-1in}%

\usepackage{authblk}
\usepackage{natbib}
\usepackage{amssymb}
\usepackage{bm}
\usepackage{amsmath}
\usepackage{booktabs}
\usepackage{multirow}
\usepackage{appendix}
\usepackage{rotating}
\usepackage{mathtools}
\usepackage{graphicx}
\usepackage{algorithm}
\usepackage{algorithmic}
\usepackage{xcolor}
\usepackage{afterpage}

\usepackage{amsthm}

% Redefine section numbering to use "S" before the section numbers

% \renewcommand{\thetable}{S\arabic{table}}
% \renewcommand{\thefigure}{S\arabic{figure}}

\usepackage{changes}
\setdeletedmarkup{\color{red}\sout{#1}}
\usepackage{cancel}

\begin{document}

\def\spacingset#1{\renewcommand{\baselinestretch}%
{#1}\small\normalsize} \spacingset{1}
\spacingset{1}

{
  \title{\bf Supplementary Materials} % for submission
  \author{}
  \date{}
  % \title{\bf Supplementary Materials \\[0.5em]
  % Space-Filling One-Factor-At-A-Time Designs}
  % \author{Wei-Yang Yu}
  % \author{V. Roshan Joseph\thanks{Corresponding author: roshan@gatech.edu}}
  % \affil{H. Milton Stewart School of Industrial and Systems Engineering, \\
  %       Georgia Institute of Technology, Atlanta, GA 30332}
  \maketitle
}

\spacingset{1}
\section{Proofs}
\subsection{Proof of Proposition 1}
\label{app:Proof pairs of levels}
\begin{proof}
Since the $2l$ levels are equally spaced, any perturbation magnitude must take the form
\[
\Delta = m\delta
\]
for some integer $m \ge 1$.
Let $(u_j, v_j)$ be a pair with $v_j - u_j = \Delta$. 
Denote $u_{\max} = \max_j u_j$. 
Because there are $l$ disjoint pairs formed from $2l$ ordered levels,
\[
u_{\max} \ge a + (l-1)\delta.
\]
For the corresponding element $v_{\max}$, we must have
\[
v_{\max} = u_{\max} + m\delta \le a + (2l-1)\delta,
\]
since $a+(2l-1)\delta$ is the largest available level. Combining the two inequalities gives
\[
a + (l-1)\delta + m\delta \le a + (2l-1)\delta,
\]
which implies
\[
m \le l.
\]
Therefore, 
\[
\sum_{j=1}^l |u_j - v_j|
\]
is maximized when $\Delta = l\delta$.
This bound is achieved by pairing
\[
(u_j, v_j) = \bigl(a + k\delta,\; a + (k+l)\delta\bigr),
\qquad k=0,1,\dots,l-1.
\]
\end{proof}

\subsection{Proof of Proposition 2}
\label{app:one-dimensional mMSEc}
\begin{proof}
    Consider a product correlation function $R(\mathbf{x}, \mathbf{x}') = \prod_{i=1}^p R(x_i, x_i')$. Let $L_i$ denote the set of $2l$ levels for the $i$th factor, and let $\bm{D}^*$ denote the corresponding full factorial design, 
    \[
    \bm{D}^* = \times_{i=1}^p L_i,
    \]
    where $\times$ denotes the Cartesian product. Then, $\mathbf{R}^* = \otimes_{i=1}^p \mathbf{R}_i$ and $\mathbf{r}^*(\mathbf{x}) = \otimes_{i=1}^p \mathbf{r}_i(x_i)$, where $\mathbf{R}_i = \{R(L_{ij}, L_{ik})\}_{j,k = 1}^{2l}$, $\mathbf{r}_i(x_i) = \{R(x_i, L_{ij})\}_{j=1}^{2l}$, and $\otimes$ denotes Kronecker product. By using the properties of Kronecker product, we have
    \begin{align*}
        \mathbf{r}^*(\mathbf{x})' \mathbf{R}^*{^{-1}} \mathbf{r}^*(\mathbf{x}) &= (\otimes_{i=1}^p \mathbf{r}_i(x_i))' (\otimes_{i=1}^p \mathbf{R}_i)^{-1} (\otimes_{i=1}^p \mathbf{r}_i(x_i)) \\
        &= (\mathbf{r}_1(x_1)' \otimes \cdots \otimes \mathbf{r}_p(x_p)') (\mathbf{R}_1^{-1} \otimes \cdots \otimes \mathbf{R}_p^{-1}) (\mathbf{r}_1(x_1) \otimes \cdots \otimes \mathbf{r}_p(x_p))\\
        &= (\mathbf{r}_1(x_1)' \mathbf{R}_1^{-1} \mathbf{r}_1(x_1)) \otimes \cdots \otimes (\mathbf{r}_p(x_p)' \mathbf{R}_p^{-1} \mathbf{r}_p(x_p))\\
        &= \prod_{i=1}^p \mathbf{r}_i(x_i)' \mathbf{R}_i^{-1} \mathbf{r}_i(x_i).
    \end{align*}
    Thus, 
    \begin{align*}
        Q(\bm{D}^*; \bm{\alpha}, \bm{\theta}) &= \min_{\mathbf{x} \in \mathcal{X}} \{ \mathbf{r}^*(\mathbf{x})' \mathbf{R}^*{^{-1}} \mathbf{r}^*(\mathbf{x}) \} \\
        &= \prod_{i=1}^p \min_{x_i} \mathbf{r}_i(x_i)' \mathbf{R}_i^{-1} \mathbf{r}_i(x_i)\\
        &= \prod_{i=1}^p q(L_i; \alpha_i, \theta_i).
    \end{align*}
    Because $\bm{D} \subset \bm{D}^*$, we can derive
    \begin{equation*}
        Q(\bm{D}; \bm{\alpha}, \bm{\theta}) \leq Q(\bm{D}^*; \bm{\alpha}, \bm{\theta}) = \prod_{i=1}^p q(L_i; \alpha_i, \theta_i).
    \end{equation*}
    Assume $\bm{D}$ is $\epsilon$-optimal with respect to $\bm{D}^*$, i.e.,
    \begin{equation*}
        Q(\bm{D}; \bm{\alpha}, \bm{\theta}) \geq (1-\epsilon)Q(\bm{D}^*; \bm{\alpha}, \bm{\theta}) = (1-\epsilon) \prod_{i=1}^p q(L_i; \alpha_i, \theta_i).
    \end{equation*}
    Then, we have
    \begin{equation*}
        (1-\epsilon) \prod_{i=1}^p q(L_i; \alpha_i, \theta_i) \leq Q(\bm{D}; \bm{\alpha}, \bm{\theta}) < \prod_{i=1}^p q(L_i; \alpha_i, \theta_i).
    \end{equation*}
    Thus, maximizing $\prod_{i=1}^p q(L_i; \alpha_i, \theta_i)$ raises both lower and upper bounds of $Q(\bm{D}; \bm{\alpha}, \bm{\theta})$.
\end{proof}

\newpage
\spacingset{1}
\section{Benchmark Functions in Numerical Studies}

\subsection{G-function}
It is defined as
\begin{equation*}
    f(\mathbf{x}) = \prod_{i=1}^{8} \frac{|4x_i - 2| + a_i}{1 + a_i},
\end{equation*}
where $x_1, \dots, x_8 \in [0,1]$, $a_1 = a2 = 0$ and $a_3 = \cdots a_8 = 3$.

\subsection{Levy Function}
It is defined as
\begin{equation*}
f(\mathbf{x}) = \sin^2(\pi w_1) 
+ \sum_{i=1}^{7} (w_i - 1)^2 \left[ 1 + 10 \sin^2(\pi w_i + 1) \right] 
+ (w_8 - 1)^2 \left[ 1 + \sin^2(2\pi w_8) \right],
\end{equation*}
where
\begin{equation*}
w_i = 1 + \frac{x_i - 1}{4}, \quad \text{for all } i = 1, \dots, 8,
\end{equation*}
and $x_1, \dots, x_{8} \in [0,1]$.

\subsection{Ackley Function}
It is defined as
\begin{equation*}
f(\mathbf{x}) = -a \exp\left( -b \sqrt{\frac{1}{8} \sum_{i=1}^8 x_i^2} \right)
- \exp\left( \frac{1}{8} \sum_{i=1}^8 \cos(c x_i) \right)
+ a + \exp(1),
\end{equation*}
where
$a = 20$, $b = 0.2$, $c = 2\pi$, and $x_1, \dots, x_{8} \in [-32.768,32.768]$.

\subsection{Borehole Function}
The function models water flow through a borehole.
It is defined as
\begin{align*}
f(\mathbf{x}) = \frac{2\pi T_u (H_u - H_l)}
{\ln(r / r_w)\left(1 + \frac{2 L T_u}{\ln(r / r_w)\, r_w^2 K_w} + \frac{T_u}{T_l}\right)}.
\end{align*}
The details of input factors are summarized in Table~\ref{tab:borehole}.
\begin{table}[ht]
\centering
\caption{The input factors and their ranges in the borehole function.}
\begin{tabular}{ll}
\hline
$r_w \in [0.05, 0.15]$ & radius of borehole (m) \\
$r \in [100, 50{,}000]$ & radius of influence (m) \\
$T_u \in [63{,}070, 115{,}600]$ & transmissivity of upper aquifer (m$^2$/yr) \\
$H_u \in [990, 1110]$ & potentiometric head of upper aquifer (m) \\
$T_l \in [63.1, 116]$ & transmissivity of lower aquifer (m$^2$/yr) \\
$H_l \in [700, 820]$ & potentiometric head of lower aquifer (m) \\
$L \in [1120, 1680]$ & length of borehole (m) \\
$K_w \in [9855, 12045]$ & hydraulic conductivity of borehole (m/yr) \\
\hline
\end{tabular}
\label{tab:borehole}
\end{table}

\newpage
\subsection{Robot Arm Function}
The function models a four-segment robotic arm with the shoulder fixed at the origin. Segment $i$ has length $L_i$ and orientation angle $\theta_i$, $i=1,\dots,4$. The output is the distance from the end of the robot arm to the origin. 
The details of input factors are summarized in Table~\ref{tab:robot}.
\begin{table}[h]
\centering
\caption{The input factors and their ranges in the robot arm function.}
\label{tab:robot}
\begin{tabular}{ll}
\hline
$\theta_1 \in [0, 2\pi]$ & Angle of the first arm segment \\
$\theta_2 \in [0, 2\pi]$ & Angle of the second arm segment \\
$\theta_3 \in [0, 2\pi]$ & Angle of the third arm segment \\
$\theta_4 \in [0, 2\pi]$ & Angle of the fourth arm segment \\
$L_1 \in [0, 1]$ & Length of the first arm segment \\
$L_2 \in [0, 1]$ & Length of the second arm segment \\
$L_3 \in [0, 1]$ & Length of the third arm segment \\
$L_4 \in [0, 1]$ & Length of the fourth arm segment \\
\hline
\end{tabular}
\end{table}

It is defined as 
\[
f(\mathbf{x}) = \left(u^2 + v^2\right)^{0.5},
\]
where
\[
u = \sum_{i=1}^{4} L_i \cos\left( \sum_{j=1}^{i} \theta_j \right),
\]
\[
v = \sum_{i=1}^{4} L_i \sin\left( \sum_{j=1}^{i} \theta_j \right).
\]

\subsection{Dette \& Pepelyshev Function}
It is defined as
\begin{align*}
f(\mathbf{x}) 
= 4\left(x_1 - 2 + 8x_2 - 8x_2^2\right)^2
+ (3 - 4x_2)^2
+ 16 \sqrt{x_3 + 1}\,(2x_3 - 1)^2
+ \sum_{i=4}^{8} i \ln\left(1 + \sum_{j=3}^{i} x_j \right).
\end{align*}
where $x_1, \dots, x_{8} \in [0,1]$.

\newpage
\spacingset{1}
\section{Additional Benchmark Functions}
\begin{figure}[ht!]
    \centering
    \includegraphics[scale=0.0417] {all_mse_panels_2.jpeg}
    \caption{Out-of-sample log MSE for the Borehole, Robot Arm, and Dette \& Pepelyshev functions under varying input dimensions. The GP surrogate model uses the MIM kernel.}
    \label{fig:all_mse_panels_2}
\end{figure}

\newpage
\spacingset{1}
\section{Additional Results using Gaussian Kernel}

\begin{figure}[ht!]
    \centering
    \includegraphics[scale=0.0417] {GP_all_mse_panels.jpeg}
    \caption{Out-of-sample log MSE for the G-function, Levy, and Ackley functions under varying input dimensions. The GP surrogate model uses the Gaussian kernel.}
    \label{fig:GP_all_mse_panels}
\end{figure}

\begin{figure}[ht!]
    \centering
    \includegraphics[scale=0.0417] {GP_all_mse_panels_2.jpeg}
    \caption{Out-of-sample log MSE for the Borehole, Robot Arm, and Dette \& Pepelyshev functions under varying input dimensions. The GP surrogate model uses the Gaussian kernel.}
    \label{fig:GP_all_mse_panels_2}
\end{figure}

\end{document}
